# Supplementary material for: Self-consistent scheme for optical response of large hybrid networks of semiconductor quantum dots and plasmonic metal nanoparticles
Source: arXiv:1606.04484 source file (2016-06-14)
Supplement: Supplementary file 1 [file Supplementary_Material_arxiv.pdf]

# Supplementary Material: A Self-Consistent Scheme for Optical Response of Large Hybrid Networks of Semiconductor Quantum Dots and Plasmonic Metal Nanoparticles

L. Hayati[1], C. Lane[2], B. Barbiellini[2], A. Bansil[2], and H. Mosallaei[1]

[1]CEM and Photonics Lab, Electrical and Computer Engineering Department, Northeastern University, Boston 02115, USA,
[2]Physics Department, Northeastern University Boston MA 02115, USA

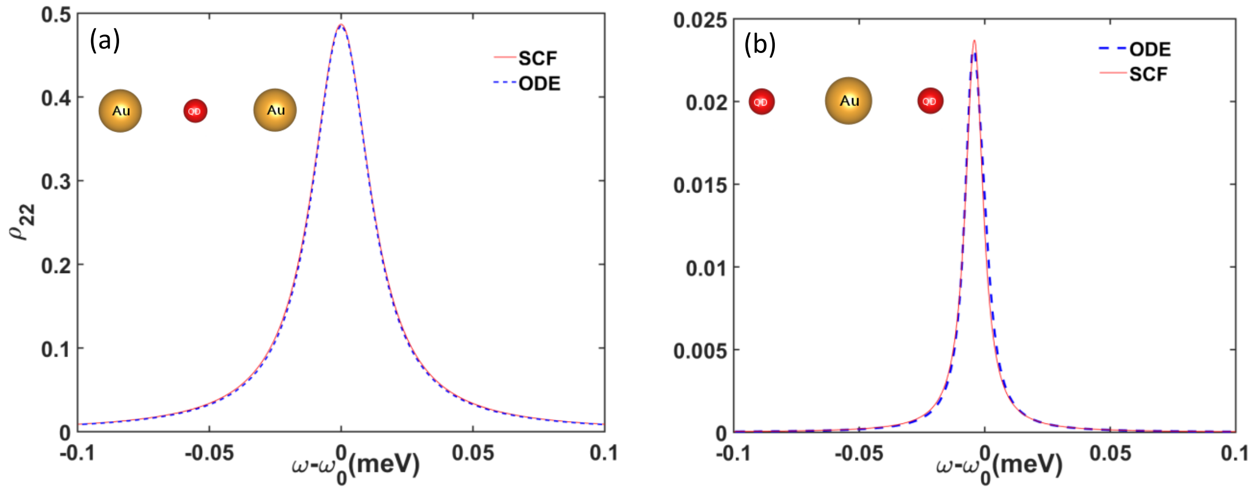


Fig. S1: Population of excited states for two different trimers using ODE and SCF methods. Good accord is seen between the results based on the two methods. (a) A MNP-SQD-MNP trimer with: center-to-center distance R = 20 nm, MNP radius a = 3 nm, dipole moment of QDOT: μ = 0.25 e nm, and light intensity of $10^3$ w/cm$^2$. (b) A SQD-MNP-SQD trimer with: center-to-center distance R=20 nm, MNP radius a = 7.5 nm, dipole moment of QDOTs: μ = 0.5 e nm, and light Intensity of 1 w/cm$^2$.

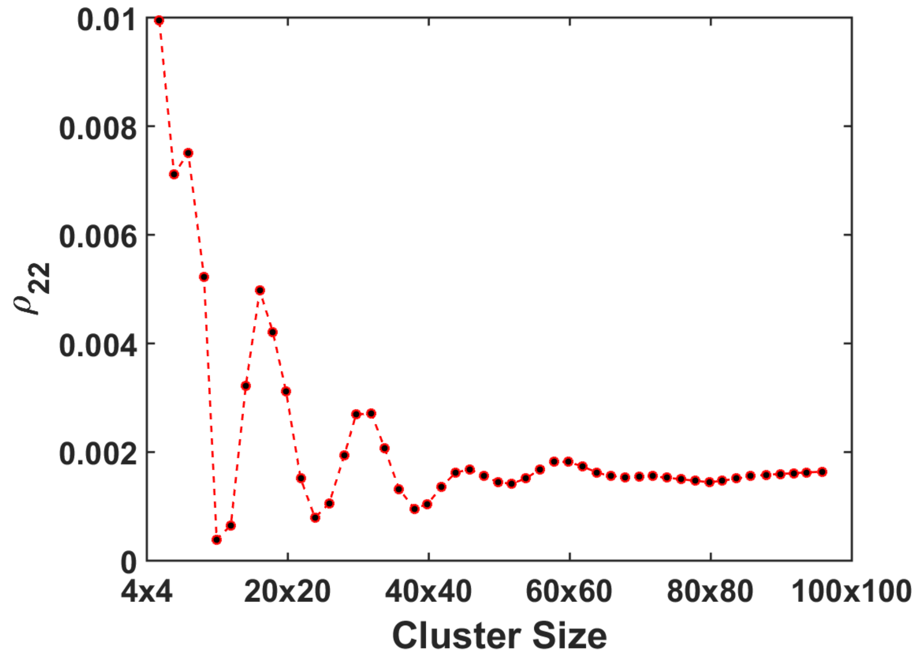


Fig. S2: Population of the excited states for the central SQD as a function of lattice (square) size at the frequency $\omega=\omega_0$. The convergence is reached for systems greater than 80x80.

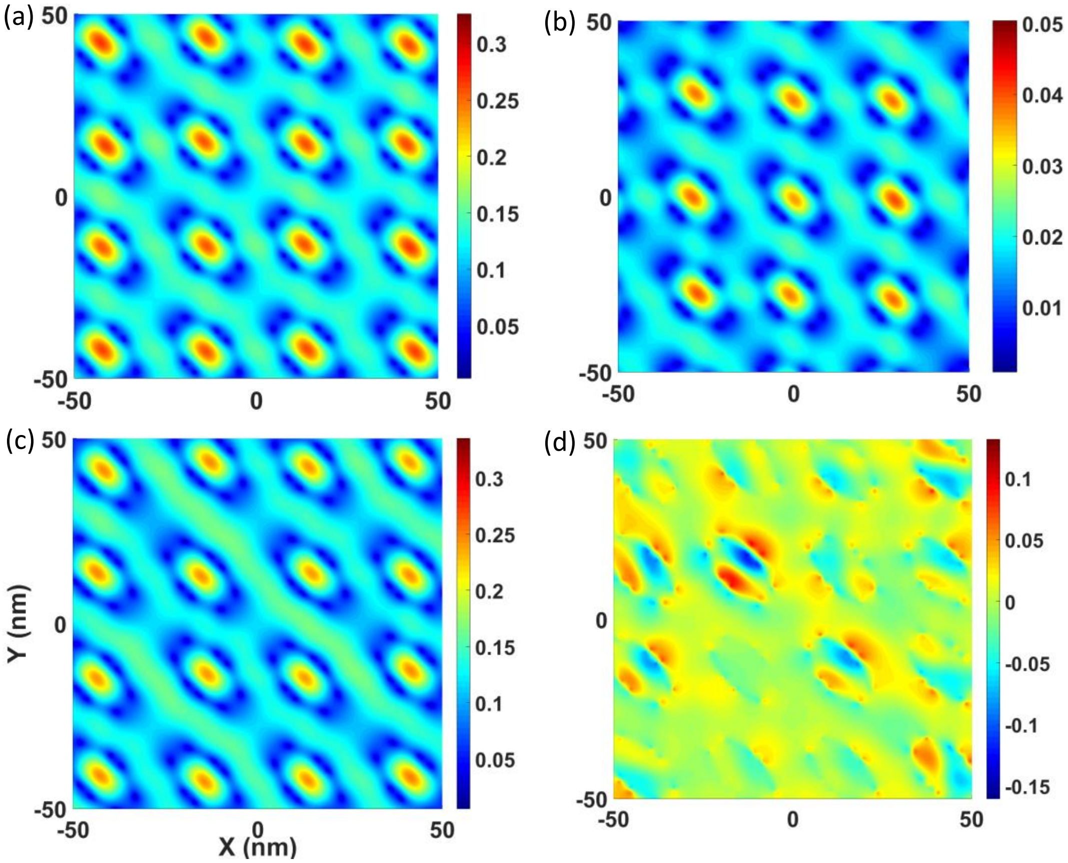


Fig. S3: Effects of disorder on the results of Fig. 4 in the main text, where the disorder is simulated by randomly varying the positions of the SQDs and MNPs in the lattice by up to 5% of the inter-particle distance away from the perfect lattice positions.

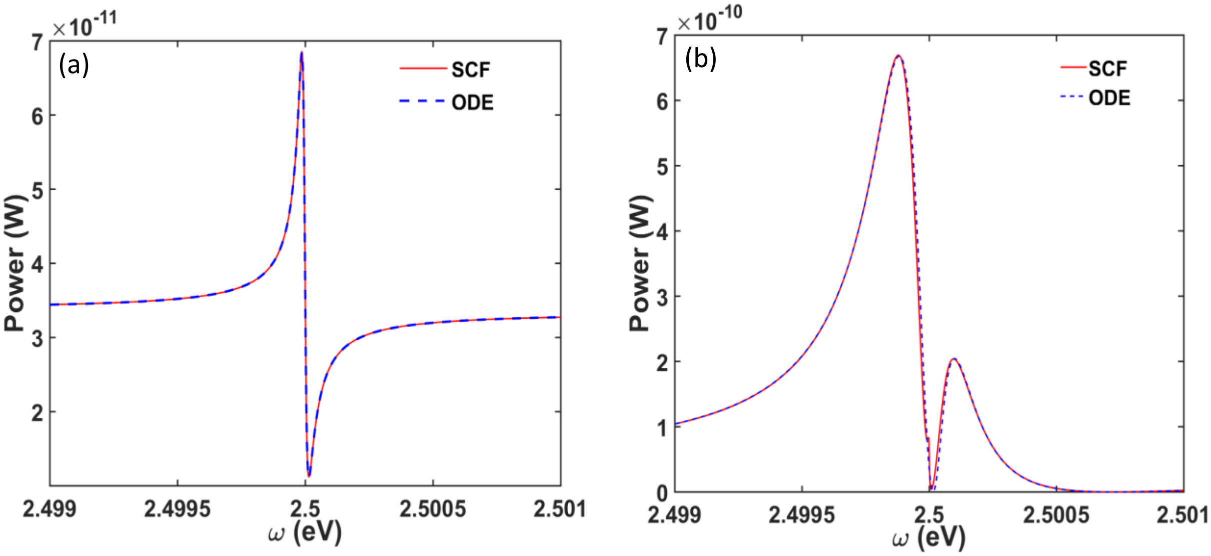


Fig. S4: Absorption power of the MNP in the dimer case [R=13 nm; a=3 nm; and, light intensity=103 W/cm2]: (a) Fano shape for μ=0.25 e nm, and (b) shows plexitonic effects, such as a EIT and the modified Fano shape, for μ=2 e nm.
